# Supplementary material for: View-Based Owicki-Gries Reasoning for Persistent x86-TSO (Extended Version)
Source: arXiv:2201.05860 source file (2022-01-15)
Supplement: Supplementary file 1 [file appendix-WF.tex]

\section{Well formedness}

 \newcommand{\maxvp}{{\sf maxvp}}
 \newcommand{\maxcoh}{{\sf maxcoh}}

  \BD{Move to sect 5?}

 Let
 $ts.\maxvp[l] = (\sqcup_{l}~ ts.\xxcoh[l]) \sqcup \xxper$ and
 and
 $ts.\maxcoh = \sqcup_{l}~ ts.\xxcoh[l]$ and
 
 We say $(T, M)$ is well formed if:
 \begin{align}
   & M \neq [\,] \wedge head(M) = initMsg \wedge
   (\forall i.\ i>0 \wedge i<|M| \Rightarrow M(i) \neq initMsg)
   \\
   & \forall t, l.\   
   \begin{array}[t]{@{}l@{}}
     {\sf let}\ ts = T.t\ {\sf in } \\
     0 \leq ts.\vrp, ts.\vpp, ts.\xxcoh[l], ts.\xxpera[l], ts.\xxper[l] <  |M|
     \wedge {}
     \\
     0 \leq \maxcoh, ts.\maxvp[l]   < |M|
     \wedge {} 
   ts.\xxcoh[l], ts.\vrp \leq ts.\maxcoh[l] \wedge {} \\
   ts.\xxper[l] \leq ts.\maxvp[l] \wedge
   ts.\vrp \leq  ts.\vpp
   \end{array}
   \\
   & \forall t, l.\ T[t].\xxcoh[l] \neq 0 \imp
     (M[T[t].\xxcoh[l]]).loc = l
   \\
   & (\forall t, l.
   \begin{array}[t]{@{}l@{}}
   ts.OTS_t(l) \neq \emptyset \wedge  
   ts.OPTS(l) \neq \emptyset \wedge  
   ts.OATS_t(l) \neq \emptyset ) \wedge {} \\ 
   ts.\View{l}{t} \neq \emptyset \wedge ts.\PView{l} \neq \emptyset \wedge ts.\AView{l}{t} \neq \emptyset) 
   \end{array}
 \end{align}

 \BD{Not sure we want all of these.}
% \begin{verbatim}
% definition "mem_structured ts  ≡ memory ts ≠ [] \wedge  (memory ts !0)=Init_Msg ∧
%                                   (∀i.(i>0∧i<length(memory ts))⟶(memory ts !i)≠Init_Msg)"

% definition 
% "vbounded ts  ≡
% (∀ ti addr. 0 ≤ vrnew ts ti ∧ vrnew ts ti  <  length (memory ts)∧
%             0 ≤ vpready ts ti ∧vpready ts ti <  length (memory ts) ∧
%             0 ≤ coh ts ti addr ∧  coh ts ti addr <  length (memory ts) ∧
%             0 ≤  vpasync ts ti addr ∧  vpasync ts ti addr <  length (memory ts) ∧
%             0 ≤  vpcommit ts ti addr ∧  vpcommit ts ti addr <  length (memory ts) ∧
%             0 ≤  maxcoh ts ti ∧  maxcoh ts ti < length (memory ts) ∧
%             0 ≤  maxvp ts addr  ∧ maxvp ts addr  < length (memory ts) ∧ 
%             coh ts ti addr ≤ maxcoh  ts ti ∧
%             vpcommit ts ti addr ≤ maxvp ts addr ∧
%             vrnew ts ti ≤  maxcoh ts ti ∧ 
%             vrnew ts ti ≤  vpready ts ti
%      ) " 

% definition  "coh_loc_rel  ts  ≡
% ∀ti l. comploc ( (memory ts)!(coh ts ti l)) l = l"

% definition "total_OTSF s ≡  ∀  nview ti l . OTSF s ti l nview ≠ {}"

% definition " total_wfs ts  ≡
%        vbounded ts ∧
%        mem_structured ts ∧
%         total_OTSF ts ∧
%       ( ∀ ti l. (comploc ( (memory ts)!(coh ts ti l)) l = l ∧
%            OTS  ts ti  l ≠ {}∧
%            OPTS ts  l ≠ {} ∧
%            OATS  ts ti  l ≠ {} ) ∧
%            [l]⇩ti ts ≠ {} /\ [l]_P ts != {} /\ [l]^A_ti ts != {})  "

% \end{verbatim}
